# Supplementary material for: SkipSNN: Efficiently Classifying Spike Trains with Event-attention
Source: arXiv:2411.05806 source file (2024-10-29)
Supplement: Supplementary file 1 [file 09_appendix.tex]

\appendix
\section{Appendix for reproducibility}
\label{sec:appendix}

This section provides more detail of datasets preprocessing, baseline settings and visual comparison to support the reproducibility of the results in this paper. We have released our code and data publicly available at Github:~\url{https://github.com/anonymous3214/ABN}.

\subsection{Details of Data Preprocessing}
For the 2D face image registration task, we conduct experiments using Flickr-Faces-HQ (FFHQ) dataset.
We collect the pairs of source images and target images by applying random deformation to the raw image. Each image is dealigned using a random deformation field smoothed by a Gaussian filter. We set the standard deviation for Gaussian kernel, $\sigma$ = 18, and a scale factor of displacement, $\alpha$ = 800, to ensure a reasonable deformation.

For the 3D brain MRI registration task, we conduct experiments on two public brain MRI datasets, LPBA40 and Mindboggle101. All scans are resized to $96\times96\times96$ with 1mm isotropic voxels. Standard pre-processing steps have been completed in both datasets, including brain extraction and affine spatial normalization. Table \ref{tab:dataset} summarizes the properties of datasets.
\input{tab_datasets}

\subsection{Detailed Settings of Baselines}
\noindent\textbullet\ \textbf{Affine}: 
This method breaks the image registration task into a composition of a linear transformation and a translation. We use existing affine implementation in the publicly available software package - ANTsPy~$\footnote{https://github.com/ANTsX/ANTsPy\label{ants}}$ with the default setting.

\noindent\textbullet\ \textbf{BSpline}: This method uses control points and spline functions to describe the nonlinear geometric transformation domain. We use existing BSpline implementation in the publicly available software package - SimpleITK (SITK)~$\footnote{https://simpleitk.org/\label{sitk}}$. Each pair of images is optimized with a order of 3, and a gradient tolerance of $1 \times 10^{-10}$ for 200 iterations.

\noindent\textbullet\ \textbf{Demons}: This method is inspired by the optical flow equations and considers non-rigid image registration as a diffusion process. We use existing Demons implementation in the publicly available software package - SimpleITK (SITK)~$\textsuperscript{\ref {sitk}}$. Each pair of images is optimized with a smooth regularization of 2, and a gradient tolerance of $1 \times 10^{-10}$ for 50 iterations.

\noindent\textbullet\ \textbf{Elastic}: This method estimates the elastic geometric deformation by updating transformation parameters iteratively. Elastic is included in the ANTsPy~$\textsuperscript{\ref {ants}}$ software package. We run the elastic registration with the default setting.

\noindent\textbullet\ \textbf{SyN}: This is a top-performing traditional method for deformable image registration. This method optimizes the space of diffeomorphic maps by maximizing the cross-correlation between images. 
We run SyN via ANTsPy~$\textsuperscript{\ref {ants}}$ with a default setting.

\noindent\textbullet\ \textbf{VM}: This is an unsupervised single-stage registration method, which uses one network to predict the deformation between images. For network architectures, we use the latest version, VoxelMorph-2, and configure 10 convolutional layers with 16, 32, 32, 64, 64, 64, 32, 32, 32 and 16 filters. The kernel size of each convolutional layer is $3 \times 3$. The ratio of regularization is set to $\lambda=10$.

\noindent\textbullet\ \textbf{CRN}:
This is a state-of-the-art learning-based method for unsupervised image registration with a multi-stage design. In different stages, the source image is repeatedly deformed to align with a target image. The number of stages is set to 10. In each stage, we configure 10 convolutional layers with 16, 32, 32, 64, 64, 64, 32, 32, 32 and 16 filters. The kernel size of each convolutional layer is $3 \times 3$. The ratio of regularization is set to $\lambda=10$.

\noindent\textbullet\ \textbf{ABN-L}: ABN-L is a variant of ABN, which only contains a long-term memory network at each stage. The network handles the registration and combination of deformations simultaneously. The number of stages is set to 10. The long-term memory network has 3 inputs, thus we increase the filters of convolutional layers to 32, 64, 64, 128, 128, 128, 64, 64, 64, and 32. The kernel size of each convolutional layer is $3 \times 3$. The ratio of regularization is set to $\lambda=10$.

\noindent\textbullet\ \textbf{ABN}:
This is our proposed model which consists of two sub-networks at each stage, the short-term registration and long-term memory networks.
The number of stages is set to 10.
We configure 10 convolutional layers in each sub-network with 16, 32, 32, 64, 64, 64, 32, 32, 32 and 16 filters. The kernel size of each convolutional layer is $3 \times 3$. The ratio of regularization is set to $\lambda=10$.

%\subsection{Visual comparison on 3D Brain MRI Registration}
%We provide a comprehensive visual comparison of the 3D brain MRI registration task on the Mindboggle101 dataset in Figure~\ref{fig:mind}. This comparison indicates that our  proposed method ABN achieves a higher level of  registration accuracy while preserving image sharpness more effectively.

\balance
